# Supplementary material for: Platonic Polyhedra, Topological Constraints and Periodic Solutions of the Classical $N$-Body Problem
Source: arXiv:0903.1397 source file (2009-03-08)
Supplement: Supplementary file 1 [file platorb_appendix.tex]

% ========================================
\section{Test orbits}

% ------------------------------------------------------
\subsection{\sc Tetrahedron}
We describe 1/6 of the orbit.
\[
\omega_2(\rho) = \frac{1}{2\rho^{3/2}}\,;
\hskip 1cm
\omega_3(\rho) = \frac{\sqrt{3}}{(\frac{\ell}{2}-\rho)^{3/2}}\,;
\]

%\begin{figure}
%\centerline{\epsfig{figure=figures/tetra_link1_init.ps,width=10cm}}
%\centerline{\epsfig{figure=figures/tetra_link2_init.ps,width=10cm}}
%\end{figure}

% ---------------------------
{\sc $\K_1$ orbit}

\[
1 = T = 3\pi\left(\frac{1}{\omega_2} + \frac{4}{3\omega_3} \right)\,;
\]
\[
\alpha(t) = -\omega_2\,t\,;\hskip 0.4cm
\beta(t) = \omega_3\,(t-t_B)\,;\hskip 0.4cm
t_A=0\,;\hskip 0.4cm
t_B=\frac{\pi}{2\omega_2}\,;\hskip 0.4cm
t_C=t_B+\frac{2\pi}{3\omega_3}\,;
\]

\[
\bu(t_A) = \left(
\begin{array}{c}
\frac{\ell}{2\sqrt{2}}\cr
0\cr
-\rho\cr
\end{array}
\right)\,;
\hskip 0.4cm
\bvh = \left(
\begin{array}{c}
1\cr
0\cr
0\cr
\end{array}
\right)\,;
\hskip 0.4cm
\bu(t_B) = \left(
\begin{array}{c}
\frac{\ell}{2\sqrt{2}}\cr
\rho\cr
0\cr
\end{array}
\right)\,;
\hskip 0.4cm
\bwh = \frac{1}{\sqrt{3}}\left(
\begin{array}{c}
1\cr
\sqrt{2}\cr
0\cr
\end{array}
\right)\ .
\]

\medbreak
% ----------------------------
{\sc $\K_2$ orbit}
\[
1 = T = 2\pi\left(\frac{1}{\omega_3(\rho)} + \frac{2}{\omega_3(r)} \right)\,;
\]
with $r = \sqrt{3}/9(\ell-\sqrt{3}\rho)$.
\[
\alpha(t) = -\omega_3(\rho)\,t\,;\hskip 0.4cm
\beta(t) = \omega_3(r)\,(t-t_B)\,;\hskip 0.4cm
t_A=0\,;\hskip 0.4cm
t_B=\frac{\pi}{3\omega_3(\rho)}\,;\hskip 0.4cm
t_C=t_B+\frac{2\pi}{3\omega_3(r)}\,;
\]

\[
\bu(t_A) = \left(
\begin{array}{c}
\frac{\ell}{6\sqrt{2}} + \sqrt{\frac{2}{3}}\rho \cr
0\cr
-\frac{\ell}{6} + \frac{\rho}{\sqrt{3}}\cr
\end{array}
\right)\,;
\hskip 0.4cm
\bvh = \frac{1}{\sqrt{3}}\left(
\begin{array}{c}
1\cr
0\cr
-\sqrt{2}\cr
\end{array}
\right)\,;
\]
\[
\bu(t_B) = \left(
\begin{array}{c}
\frac{\ell}{6\sqrt{2}} + \frac{\rho}{\sqrt{6}} \cr
\frac{\sqrt{3}}{2}\rho\cr
-\frac{\ell}{6} + \frac{\sqrt{3}}{6}\rho\cr
\end{array}
\right)\,;
\hskip 0.4cm
\bwh = \frac{1}{\sqrt{3}}\left(
\begin{array}{c}
1\cr
\sqrt{2}\cr
0\cr
\end{array}
\right)\ .
\]

\medbreak
% ---------------------------
{\sc $\K_3$ orbit}
\[
1 = T = 3\pi\left(\frac{1}{\omega_2} + \frac{2}{3\omega_3} \right)\,;
\]
\[
\alpha(t) = \omega_2\,t\,;\hskip 0.4cm
\beta(t) = -\omega_3\,(t-t_B)\,;\hskip 0.4cm
t_A=0\,;\hskip 0.4cm
t_B=\frac{\pi}{2\omega_2}\,;\hskip 0.4cm
t_C=t_B+\frac{\pi}{3\omega_3}\,;
\]

\[
\bu(t_A) = \left(
\begin{array}{c}
\frac{\ell}{2\sqrt{2}}\cr
0\cr
-\rho\cr
\end{array}
\right)\,;
\hskip 0.4cm
\bvh = \left(
\begin{array}{c}
1\cr
0\cr
0\cr
\end{array}
\right)\,;
\hskip 0.4cm
\bu(t_B) = \left(
\begin{array}{c}
\frac{\ell}{2\sqrt{2}}\cr
\rho\cr
0\cr
\end{array}
\right)\,;
\hskip 0.4cm
\bwh = \frac{1}{\sqrt{3}}\left(
\begin{array}{c}
1\cr
\sqrt{2}\cr
0\cr
\end{array}
\right)\ .
\]

%\begin{figure}
%\centerline{\epsfig{figure=figures/hexa_link1_init.ps,width=10cm}}
%\centerline{\epsfig{figure=figures/hexa_link2_init.ps,width=10cm}}
%\end{figure}

% -----------------------------------------------
\subsection{\sc Cube (Hexahedron)}
We describe 1/8 of the orbit.
\[
\omega_2 = \frac{1}{2\rho^{3/2}}\,;
\hskip 1cm
\omega_3 = \frac{\sqrt{3}}{2^{3/4}}\frac{1}{(\frac{\ell}{2}-\rho)^{3/2}}\,;
\]

% ----------------------------------
{\sc $\K_1$ orbit} *** controllare se K1 e K2 sono scambiate ***
\[
1 = T = 4\pi\left(\frac{1}{2\omega_4} + \frac{2}{3\omega_3} \right)\,;
\]
\[
\alpha(t) = -\omega_4\,t\,;\hskip 0.4cm
\beta(t) = +\omega_3\,(t-t_B)\,;\hskip 0.4cm
t_A=0\,;\hskip 0.4cm
t_B=\frac{\pi}{4\omega_2}\,;\hskip 0.4cm
t_C=t_B+\frac{\pi}{3\omega_3}\,;
\]

\[
\bu(t_A) = \frac{1}{2}\left(
\begin{array}{c}
\rho\cr
\frac{\ell}{2}\rho\cr
0\cr
\end{array}
\right)\,;
\hskip 0.4cm
\bvh = \left(
\begin{array}{c}
0\cr
1\cr
0\cr
\end{array}
\right)\,;
\hskip 0.4cm
\bu(t_B) = \frac{1}{\sqrt{2}}\left(
\begin{array}{c}
\rho\cr
\ell/\sqrt{2}\cr
\rho\cr
\end{array}
\right)\,;
\hskip 0.4cm
\bwh = \frac{1}{\sqrt{3}}\left(
\begin{array}{c}
1\cr
1\cr
1\cr
\end{array}
\right)\ .
\]

\medbreak
% ----------------------------------
{\sc $\K_2$ orbit}
\[
1 = T = 4\pi\left(\frac{1}{\omega_2} + \frac{4}{3\omega_3} \right)\,;
\]
\[
\alpha(t) = -\omega_2\,t\,;\hskip 0.4cm
\beta(t) = \omega_3\,(t-t_B)\,;\hskip 0.4cm
t_A=0\,;\hskip 0.4cm
t_B=\frac{\pi}{2\omega_2}\,;\hskip 0.4cm
t_C=t_B+\frac{2\pi}{3\omega_3}\,;
\]

\[
\bu(t_A) = \frac{1}{2}\left(
\begin{array}{c}
\ell+\sqrt{2}\rho\cr
\ell-\sqrt{2}\rho\cr
0\cr
\end{array}
\right)\,;
\hskip 0.4cm
\bvh = \frac{1}{\sqrt{2}}\left(
\begin{array}{c}
1\cr
1\cr
0\cr
\end{array}
\right)\,;
\hskip 0.4cm
\bu(t_B) = \left(
\begin{array}{c}
\ell/2\cr
\ell/2\cr
\rho\cr
\end{array}
\right)\,;
\hskip 0.4cm
\bwh = \frac{1}{\sqrt{3}}\left(
\begin{array}{c}
1\cr
1\cr
1\cr
\end{array}
\right)\ .
\]

\medbreak
% ----------------------------------
{\sc $\K_3$ orbit}
\[
1 = T = 4\pi\left(\frac{1}{\omega_2} + \frac{2}{3\omega_3} \right)\,;
\]
\[
\alpha(t) = \omega_2\,t\,;\hskip 0.4cm
\beta(t) = -\omega_3\,(t-t_B)\,;\hskip 0.4cm
t_A=0\,;\hskip 0.4cm
t_B=\frac{\pi}{2\omega_2}\,;\hskip 0.4cm
t_C=t_B+\frac{\pi}{3\omega_3}\,;
\]

\[
\bu(t_A) = \frac{1}{2}\left(
\begin{array}{c}
\ell-\sqrt{2}\rho\cr
\ell+\sqrt{2}\rho\cr
0\cr
\end{array}
\right)\,;
\hskip 0.4cm
\bvh = \frac{1}{\sqrt{2}}\left(
\begin{array}{c}
1\cr
1\cr
0\cr
\end{array}
\right)\,;
\hskip 0.4cm
\bu(t_B) = \left(
\begin{array}{c}
\ell/2\cr
\ell/2\cr
\rho\cr
\end{array}
\right)\,;
\hskip 0.4cm
\bwh = \frac{1}{\sqrt{3}}\left(
\begin{array}{c}
1\cr
1\cr
1\cr
\end{array}
\right)\ .
\]

%\begin{figure}
%\centerline{\epsfig{figure=figures/octa_link1_init.ps,width=10cm}}
%%\centerline{\epsfig{figure=figures/tetra_link2_init.ps,width=10cm}}
%\end{figure}

% --------------------------------------------
\subsection{\sc Octahedron}
We describe 1/6 of the orbit.
\[
\omega_2 = \frac{1}{2\rho^{3/2}}\,;
\hskip 1cm
\omega_4 = \frac{\sqrt{2\sqrt{2}+1}}{\sqrt[4]{2}(\frac{\ell}{2}-\rho)^{3/2}}\,;
\]

% --------------------------
{\sc $\K_1$ orbit}
\[
1 = T = 3\pi\left(\frac{1}{\omega_2} + \frac{3}{2\omega_4} \right)\,;
\]
\[
\alpha(t) = -\omega_2\,t\,;\hskip 0.4cm
\beta(t) = \omega_4\,(t-t_B)\,;\hskip 0.4cm
t_A=0\,;\hskip 0.4cm
t_B=\frac{\pi}{2\omega_2}\,;\hskip 0.4cm
t_C=t_B+\frac{3\pi}{4\omega_4}\,;
\]

\[
\bu(t_A) = \left(
\begin{array}{c}
\frac{\ell}{2\sqrt{2}}\cr
\rho\cr
\frac{\ell}{2\sqrt{2}}\cr
\end{array}
\right)\,;
\hskip 0.4cm
\bvh = \frac{1}{\sqrt{2}}\left(
\begin{array}{c}
1\cr
0\cr
1\cr
\end{array}
\right)\,;
\hskip 0.4cm
\bu(t_B) = \frac{1}{\sqrt{2}}\left(
\begin{array}{c}
\frac{\ell}{2}+\rho\cr
0\cr
\frac{\ell}{2}-\rho\cr
\end{array}
\right)\,;
\hskip 0.4cm
\bwh = \left(
\begin{array}{c}
1\cr
0\cr
0\cr
\end{array}
\right)\ .
\]

\medbreak
% -------------------------------
{\sc $\K_2$ orbit}
\centerline{***** to be computed *****}

\medbreak
% -------------------------------
{\sc $\K_3$ orbit}
\[
1 = T = 3\pi\left(\frac{1}{\omega_2} + \frac{1}{2\omega_4} \right)\,;
\]
\[
\alpha(t) = \omega_2\,t\,;\hskip 0.4cm
\beta(t) = -\omega_4\,(t-t_B)\,;\hskip 0.4cm
t_A=0\,;\hskip 0.4cm
t_B=\frac{\pi}{2\omega_2}\,;\hskip 0.4cm
t_C=t_B+\frac{\pi}{4\omega_4}\,;
\]

\[
\bu(t_A) = \left(
\begin{array}{c}
\frac{\ell}{2\sqrt{2}}\cr
-\rho\cr
\frac{\ell}{2\sqrt{2}}\cr
\end{array}
\right)\,;
\hskip 0.4cm
\bvh = \frac{1}{\sqrt{2}}\left(
\begin{array}{c}
1\cr
0\cr
1\cr
\end{array}
\right)\,;
\hskip 0.4cm
\bu(t_B) = \frac{1}{\sqrt{2}}\left(
\begin{array}{c}
\frac{\ell}{2}+\rho\cr
0\cr
\frac{\ell}{2}-\rho\cr
\end{array}
\right)\,;
\hskip 0.4cm
\bwh = \left(
\begin{array}{c}
1\cr
0\cr
0\cr
\end{array}
\right)\ .
\]

% ---------------------------------------------------
\subsection{\sc Dodecahedron}
We describe 1/10 of the orbit.
\[
\omega_2 = \frac{1}{2\rho^{3/2}}\,;
\hskip 1cm
\omega_3 = \frac{\sqrt{3}}{\left[2(\frac{\ell}{2}-\rho)\cos(\pi/5)\right]^{3/2}}\,;
\]

% ----------------------------------
{\sc $\K_1$ orbit}
\[
1 = T = 5\pi\left(\frac{1}{\omega_2} + \frac{4}{3\omega_3} \right)\,;
\]
\[
\alpha(t) = -\omega_2\,t\,;\hskip 0.4cm
\beta(t) = \omega_3\,(t-t_B)\,;\hskip 0.4cm
t_A=0\,;\hskip 0.4cm
t_B=\frac{\pi}{2\omega_2}\,;\hskip 0.4cm
t_C=t_B+\frac{2\pi}{3\omega_3}\,;
\]

\[
\bu(t_A) = \left(
\begin{array}{c}
\frac{\ell}{\sqrt{3}}\cos(\pi/5)\cr
-\rho\cr
\frac{2\ell}{\sqrt{3}}\frac{\cos^2(\pi/5)}{\sqrt{4\sin^2(\pi/5)-1}}\cr
\end{array}
\right)
\hskip 1cm
\bvh = \frac{1}{\sqrt{3}}\left(
\begin{array}{c}
\sqrt{4\sin^2(\pi/5)-1}\cr
0\cr
2\cos(\pi/5)\cr
\end{array}
\right)
\]

\[
\bu(t_B) = \left(
\begin{array}{c}
\frac{2}{\sqrt{3}}(\frac{\ell}{2}-\rho)\cos(\pi/5)\cr
0\cr
\displaystyle\frac{3\ell - 2(\ell-2\rho)\cos(\pi/5)\sqrt{4\sin^2(\pi/5)-1}}{2\sqrt{3}\sqrt{4\sin^2(\pi/5)-1}}\cr
\end{array}
\right)\,;
\hskip 1cm
\bwh = \left(
\begin{array}{c}
0\cr
0\cr
1\cr
\end{array}
\right)\ .
\]

\medbreak
% ----------------------------------
{\sc $\K_2$ orbit}
\centerline{***** to be computed *****}

\medbreak
% ----------------------------------
{\sc $\K_3$ orbit}
\[
1 = T = 5\pi\left(\frac{1}{\omega_2} + \frac{2}{3\omega_3} \right)\,;
\]
\[
\alpha(t) = \omega_2\,t\,;\hskip 0.4cm
\beta(t) = -\omega_3\,(t-t_B)\,;\hskip 0.4cm
t_A=0\,;\hskip 0.4cm
t_B=\frac{\pi}{2\omega_2}\,;\hskip 0.4cm
t_C=t_B+\frac{\pi}{3\omega_3}\,;
\]

\[
\bu(t_A) = \left(
\begin{array}{c}
\frac{\ell}{\sqrt{3}}\cos(\pi/5)\cr
\rho\cr
\frac{2\ell}{\sqrt{3}}\frac{\cos^2(\pi/5)}{\sqrt{4\sin^2(\pi/5)-1}}\cr
\end{array}
\right)
\hskip 1cm
\bvh = \frac{1}{\sqrt{3}}\left(
\begin{array}{c}
\sqrt{4\sin^2(\pi/5)-1}\cr
0\cr
2\cos(\pi/5)\cr
\end{array}
\right)
\]

\[
\bu(t_B) = \left(
\begin{array}{c}
\frac{2}{\sqrt{3}}(\frac{\ell}{2}-\rho)\cos(\pi/5)\cr
0\cr
\displaystyle\frac{3\ell - 2(\ell-2\rho)\cos(\pi/5)\sqrt{4\sin^2(\pi/5)-1}}{2\sqrt{3}\sqrt{4\sin^2(\pi/5)-1}}\cr
\end{array}
\right)\,;
\hskip 1cm
\bwh = \left(
\begin{array}{c}
0\cr
0\cr
1\cr
\end{array}
\right)\ .
\]

% ------------------------------------------------
\subsection{\sc Icosahedron}
We describe 1/6 of the orbit.
\[
\omega_2 = \frac{1}{2\rho^{3/2}}\,;
\hskip 1cm
\omega_5 = \frac{2\sin(\pi/5)}{(\frac{\ell}{2}-\rho)^{3/2}}\sqrt{1+\frac{\sqrt{2}\sin(\pi/5)}{\sqrt{1+\cos(\pi/5)}}}\,;
\]

% ----------------------------------
{\sc $\K_1$ orbit}
\[
1 = T = 3\pi\left(\frac{1}{\omega_2} + \frac{8}{5\omega_5} \right)\,;
\]
\[
\alpha(t) = -\omega_2\,t\,;\hskip 0.4cm
\beta(t) = \omega_5\,(t-t_B)\,;\hskip 0.4cm
t_A=0\,;\hskip 0.4cm
t_B=\frac{\pi}{2\omega_2}\,;\hskip 0.4cm
t_C=t_B+\frac{4\pi}{5\omega_5}\,;
\]

\[
\bu(t_A) = \frac{\ell}{4\sin(\pi/5)}\left(
\begin{array}{c}
1\cr
-\frac{4\sin(\pi/5)}{\ell}\rho\cr
\frac{1}{\sqrt{4\sin^2(\pi/5)-1}}\cr
\end{array}
\right)\,;
\hskip 0.5cm
\bvh = \frac{1}{2\sin(\pi/5)}\left(
\begin{array}{c}
\sqrt{4\sin^2(\pi/5)-1}\cr
0\cr
1\cr
\end{array}
\right)\,;
\]

\[
\bu(t_B) = \frac{1}{2\sin(\pi/5)}\left(
\begin{array}{c}
\frac{\ell}{2}-\rho\cr
0\cr
\displaystyle\frac{\ell/2 + \rho(4\sin^2(\pi/5)-1)}{\sqrt{4\sin^2(\pi/5)-1}}\cr
\end{array}
\right)\,;
\hskip 0.5cm
\bwh = \left(
\begin{array}{c}
0\cr
0\cr
1\cr
\end{array}
\right)\ .
\]

\medbreak
% ----------------------------------
{\sc $\K_2$ orbit}
\centerline{***** to be computed *****}

\medbreak
% ----------------------------------
{\sc $\K_3$ orbit}
\[
1 = T = 3\pi\left(\frac{1}{\omega_2} + \frac{2}{5\omega_5} \right)\,;
\]
\[
\alpha(t) = \omega_2\,t\,;\hskip 0.4cm
\beta(t) = -\omega_5\,(t-t_B)\,;\hskip 0.4cm
t_A=0\,;\hskip 0.4cm
t_B=\frac{\pi}{2\omega_2}\,;\hskip 0.4cm
t_C=t_B+\frac{\pi}{5\omega_5}\,;
\]

\[
\bu(t_A) = \frac{\ell}{4\sin(\pi/5)}\left(
\begin{array}{c}
1\cr
\frac{4\sin(\pi/5)}{\ell}\rho\cr
\frac{1}{\sqrt{4\sin^2(\pi/5)-1}}\cr
\end{array}
\right)\,;
\hskip 0.5cm
\bvh = \frac{1}{2\sin(\pi/5)}\left(
\begin{array}{c}
\sqrt{4\sin^2(\pi/5)-1}\cr
0\cr
1\cr
\end{array}
\right)\,;
\]

\[
\bu(t_B) = \frac{1}{2\sin(\pi/5)}\left(
\begin{array}{c}
\frac{\ell}{2}-\rho\cr
0\cr
\displaystyle\frac{\ell/2 + \rho(4\sin^2(\pi/5)-1)}{\sqrt{4\sin^2(\pi/5)-1}}\cr
\end{array}
\right)\,;
\hskip 0.5cm
\bwh = \left(
\begin{array}{c}
0\cr
0\cr
1\cr
\end{array}
\right)\ .
\]
